# Supplementary material for: Mechanochemical Topological Defects in an Active Nematic
Source: arXiv:2210.03796 ancillary file (2024-07-27)
Supplement: Supplementary file 1 [file supp.pdf]

# Mechanochemical Topological Defects in an Active Nematic

## Electronic Supplement

Michael M. Norton<sup>1,\*</sup> and Piyush Grover<sup>2</sup>

<sup>1</sup>*School of Physics and Astronomy, Rochester Institute of Technology, Rochester, New York 14623, USA*

<sup>2</sup>*Mechanical and Materials Engineering, University of Nebraska - Lincoln, Lincoln, Nebraska 68588, USA*

- **Movie S1:** Movie showing the time evolution of *case i* dynamics: (upper-left)  $\mathbf{Q}$  and  $s$ , (lower-left)  $\mathbf{u}$  and  $\omega$ , (upper-right)  $\phi$  and  $\mathbf{p}$ , (lower-right)  $\rho$ . See Table S1, row 3 for a list of all simulation parameters. The simulation begins in a nearly uniformly aligned state and evolves towards a chaotic state with several defects.
- **Movie S2:** Movie showing the time evolution for *case ii* dynamics: (upper-left)  $\mathbf{Q}$  and  $s$ , (lower-left)  $\mathbf{u}$  and  $\omega$ , (upper-right)  $\phi$  and  $\mathbf{p}$ , (lower-right)  $\rho$ . See Table S1, row 4 for a list of simulation parameters. The simulation begins in a nearly uniformly aligned state and evolves towards a chaotic state with several defects.

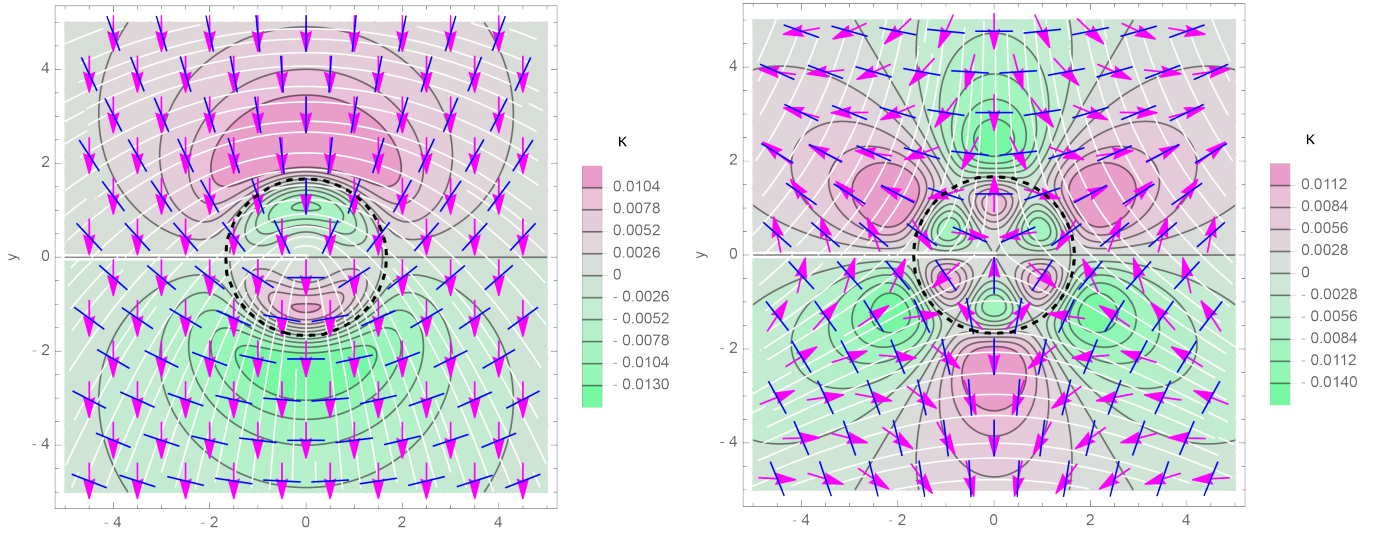

FIG. S1. **Idealized half-integer defects.** Plots show director field (white lines), vector field  $\perp \mathbf{n}$  (blue sticks), normalized  $\nabla \cdot \mathbf{Q}$  (magenta arrows), and the scalar invariant  $\kappa = Q_{ij}Q_{ik,j}Q_{kl,l}$  (color field) used to select regions of preferred bend for  $+\frac{1}{2}$  (left) and  $-\frac{1}{2}$  (right) defects. The director fields are given by the analytical expressions  $\mathbf{n}_{\pm} = \{-\cos(\frac{1}{2}(\theta - \theta_0)), \mp \sin(\frac{1}{2}(\theta - \theta_0))\}$  with  $\theta = \tan^{-1}(y/x)$  and  $\theta_0 = \pm\pi/2$  for  $\pm\frac{1}{2}$ . The nematic order tensor is given by  $\mathbf{Q} = s(\mathbf{x})[\mathbf{n} \otimes \mathbf{n} - \frac{1}{2}\mathbf{I}]$ , where the defect core is approximated using a Gaussian divot with unit standard deviation such that  $s(\mathbf{x}) = 1 - e^{-\frac{1}{2}\mathbf{x} \cdot \mathbf{x}}$ . In the model for  $\mathbf{p}$  described in the manuscript, we use two energetic terms to enforce a relationship between  $\mathbf{p}$  and  $\mathbf{Q}$ . Firstly, we wish  $\mathbf{p}$  to be essentially  $\perp \mathbf{n}$ . However, the energy we use to enforce this  $\sim (\mathbf{p} \otimes \mathbf{p}) : \mathbf{Q}$  cannot uniquely determine  $\mathbf{p}$  because it is invariant to  $\mathbf{p} \rightarrow -\mathbf{p}$ . To break this degeneracy (that is, choose a consistent direction for  $\mathbf{p}$ ), we include the term  $\sim (\nabla \cdot \mathbf{Q}) \cdot \mathbf{p}$ , which is linear in  $\mathbf{p}$  and therefore does discriminate between  $\pm\mathbf{p}$ . To choose a sign for this term, we observe that in regions of  $\kappa > 0$ ,  $\nabla \cdot \mathbf{Q}$  naturally points towards  $+\frac{1}{2}$  defects and away from  $-\frac{1}{2}$  defects. Thus, penalizing  $(\nabla \cdot \mathbf{Q}) \cdot \mathbf{p}$  causes  $\mathbf{p}$  to point in the direction opposite the magenta arrows: preferentially inward for  $-\frac{1}{2}$  defects, and outward for  $\frac{1}{2}$  defects. The contours of  $\kappa$  show that both defects exhibit similar degrees of distortion (with pink corresponding to bend-rich, and green to splay-rich regions) outside the defect cores (dashed black line corresponds to  $s = 0.75$ ).

\* mike.m.norton@gmail.com

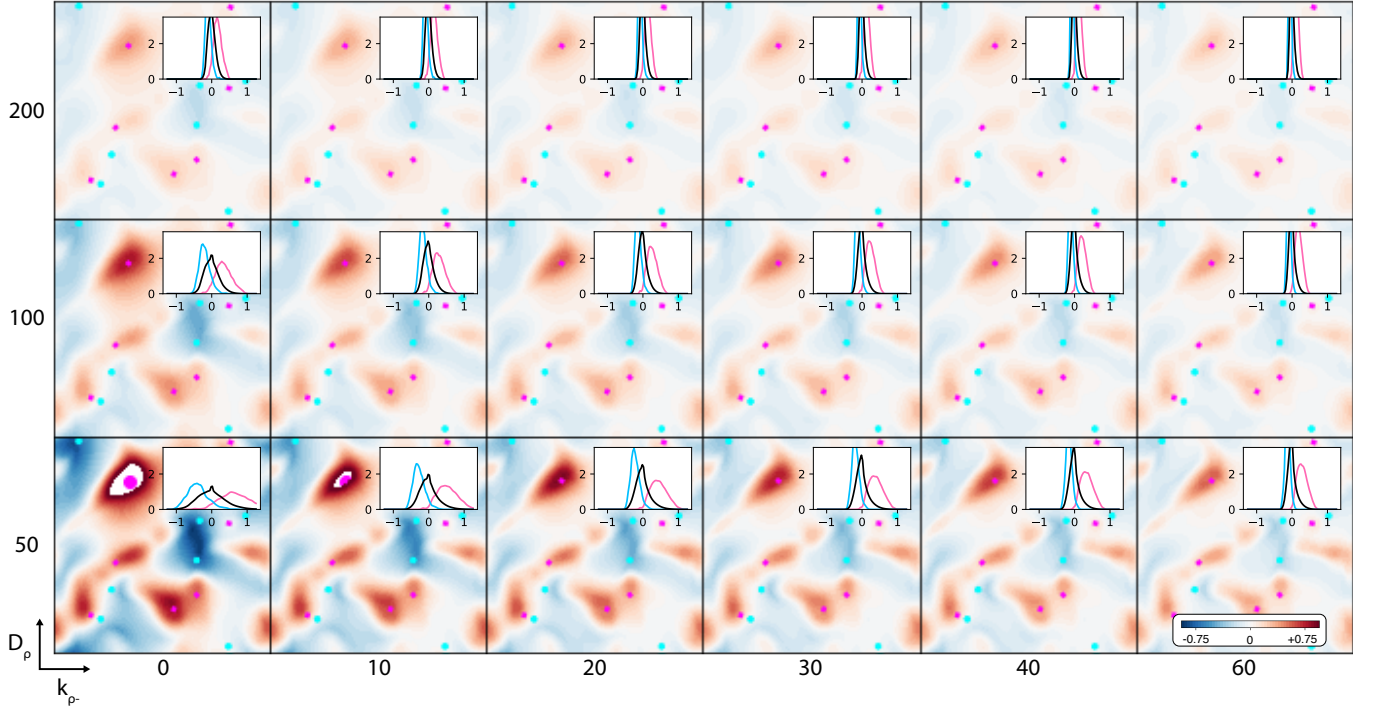

FIG. S2. **Case ii behavior of  $\rho$  without phase separation.** Here, we consider a simpler model by replacing Eqn. 7 in the main text with  $\partial_t \rho + \mathbf{u} \cdot \nabla \rho = k_{\rho+} \nabla \cdot \mathbf{p} - k_{\rho-} \rho + D_\rho \nabla^2 \rho$  (note the removal of  $\mu_\rho$ ). Frames show snapshots of  $\rho$  and insets show the probability density function of  $\rho$  for regions containing  $+\frac{1}{2}$  defects (pink),  $-\frac{1}{2}$  (blue), and no defects (black). We vary  $D_\rho$  (rows) and  $k_{\rho-}$  (columns). All other parameters are shown in Table S1, row 5. Defects continue to reside in regions of  $\rho$  matching their sign despite this change in the model. However the locations of the maxima for the blue and pink curves are not symmetric (that is  $\rho_+ \neq |\rho_-|$ ) for the two charges and the regions of  $\pm$  are not always well-defined.

|                                  | <b>u</b> |       |           | <b>Q</b>   |          | $\phi$   |       |             |              | <b>p</b>     |               |               |          |             | $\rho$      |          |           |               |       |  |
|----------------------------------|----------|-------|-----------|------------|----------|----------|-------|-------------|--------------|--------------|---------------|---------------|----------|-------------|-------------|----------|-----------|---------------|-------|--|
|                                  | $\alpha$ | $\xi$ | $\lambda$ | $\kappa_0$ | $\delta$ | $D_\phi$ | $k_0$ | $k_{\phi-}$ | $\beta_{p1}$ | $\beta_{p2}$ | $\beta_{pQ1}$ | $\beta_{pQ2}$ | $\phi_c$ | $k_{\rho+}$ | $k_{\rho-}$ | $A$      | $D_\rho$  | $\gamma_\rho$ | $s_c$ |  |
| <i>case i</i> : isolated defect  | -        | -     | -         | 1E-2       | 2E-5     | 0.02     | 15    | 2           | 15           | 1            | 15            | 1.5           | 0.5      | 15          | 5           | 0        | 7         | 0.1           | 0.6   |  |
| <i>case ii</i> : isolated defect | -        | -     | -         | 5E-3       | -        | -        | -     | -           | 15           | 1            | 15            | 1.5           | -        | 6           | 3           | 0        | 7         | 0.1           | 0.6   |  |
| <i>case i</i> : active flow      | -6       | 0.1   | 1         | 0.1        | 5E-4     | 0.1      | 200   | 10          | 50           | 1            | 50            | 5             | 0.4      | 120         | 60          | 0.15     | 100       | 0.04          | 0.8   |  |
| <i>case ii</i> : active flow     | -6       | 0.1   | 1         | 0.1        | -        | 0.1      | -     | -           | 50           | 1            | 50            | 5             | -        | 40          | 20          | 0.1125   | 100       | 0.04          | 0.8   |  |
| <i>case ii</i> : Fig. S2         | -6       | 0.1   | 1         | 0.1        | -        | 0.1      | -     | -           | 50           | 1            | 50            | 5             | -        | 40          | <b>v</b>    | -        | <b>v*</b> | -             | -     |  |
| <i>case ii</i> : Fig. S3         | -6       | 0.1   | 1         | 0.1        | -        | 0.1      | -     | -           | 50           | 1            | 50            | 5             | -        | 40          | <b>v</b>    | 0.225    | <b>v</b>  | 0.04          | 0.8   |  |
| <i>case ii</i> : Fig. S4         | -6       | 0.1   | 1         | 0.1        | -        | 0.1      | -     | -           | 50           | 1            | 50            | 5             | -        | 40          | 20          | <b>v</b> | 100       | 0.04          | 0.8   |  |

TABLE S1. Table of parameters used in simulations. Parameters are grouped according to the dynamics they control.  $\kappa_0$  is the exception, as it controls  $\phi$ -dynamics in case i and  $\mathbf{p}$ -dynamics directly for case ii. The first two rows correspond to the isolated, passive ( $\mathbf{u} = 0$ ) defects shown in Fig. 2 and the next two correspond to the full nematohydrodynamic simulations shown in Fig. 3 and Movies S1,S2. The final three rows are for simulations shown only in the supplement.  $\mathbf{v}$  indicates a parameter that is varied and \* emphasizes that  $D_\rho$  is the Fickian diffusivity rather than the Cahn-Hilliard diffusivity (see Fig. S2).

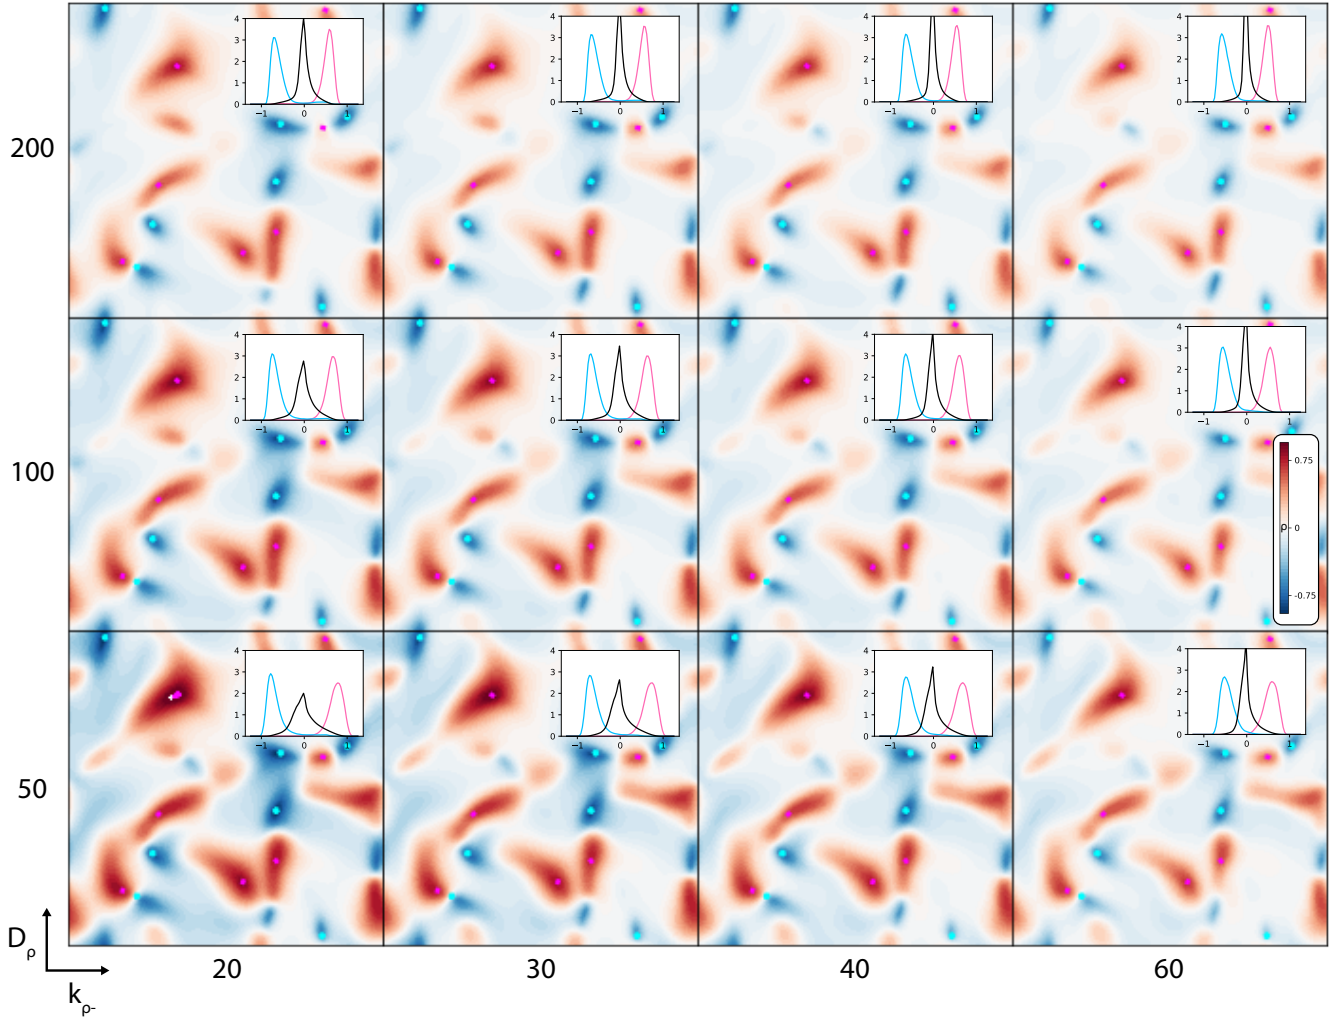

FIG. S3. **Case *ii* behavior of  $\rho$  varying mobility  $D_\rho$  and destruction rate  $k_{\rho-}$ .** Frames show snapshots of  $\rho$  and insets show the probability density function of  $\rho$  for regions containing  $+\frac{1}{2}$  defects (pink),  $-\frac{1}{2}$  (blue), and no defects (black). We vary  $D_\rho$  (rows) and  $k_{\rho-}$  (columns). All other parameters are shown in Table S1, row 6. Compared to Fig. S2, the locations and width of peaks are much less sensitive to the values for  $D_\rho$  and  $k_{\rho-}$  indicating that phase separation adds robustness to the defect detection system.

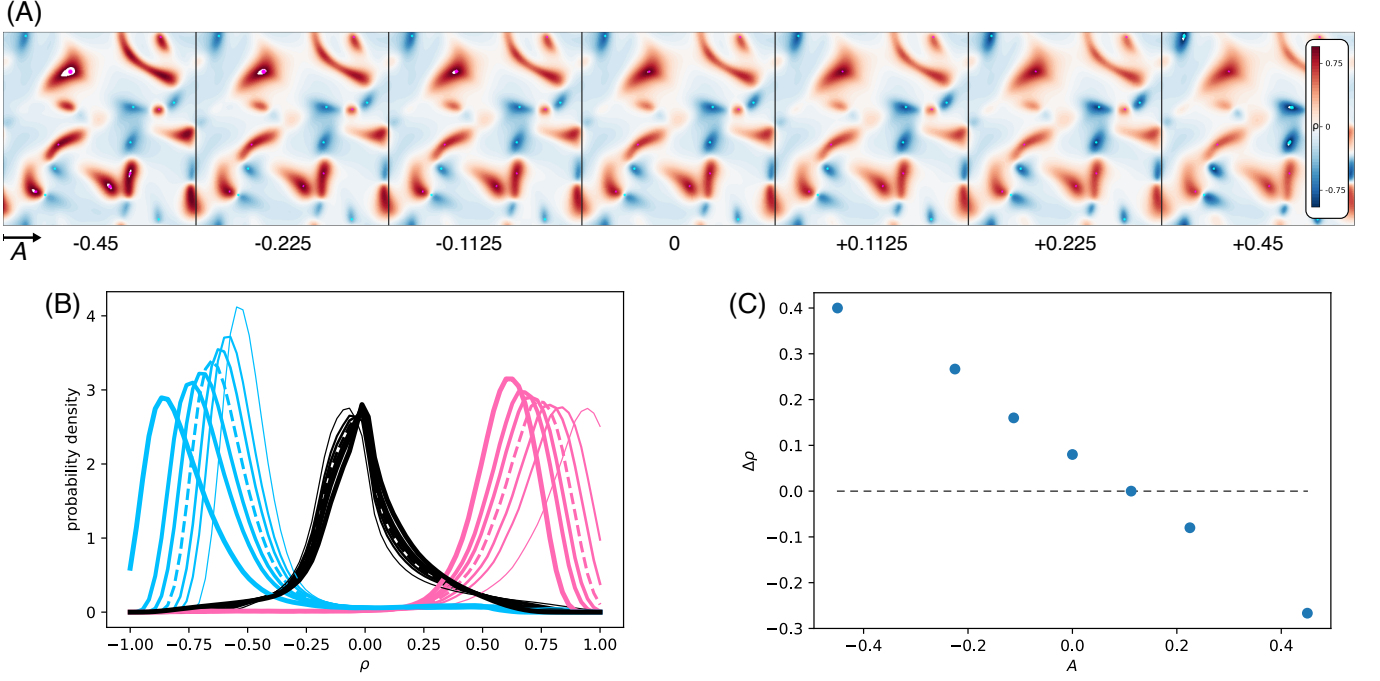

FIG. S4. **Case ii behavior of  $\rho$  while varying phase-separation roots.** (A) Representative snapshots of  $\rho$  for various  $A$  (see Eqn. 8 in the main text) while holding all other parameters fixed, Table S1, row 7. (B) The probability density function of  $\rho$  for regions containing  $+\frac{1}{2}$  defects (pink),  $-\frac{1}{2}$  (blue), and no defects (black), with line thickness indicating  $A$  (thin for small values, thick for large values, and dashed for  $A = 0$ ). The distributions shift from right to left as  $A$  is increased while leaving the distribution within neutral regions relatively unchanged. (C) The quantity  $\Delta\rho = \rho_+^* - |\rho_-^*|$  measures the degree of asymmetry between the locations of the peaks  $\rho^*$  for each distribution in (B); using  $A = 0.1125$  symmetrizes these locations.
